# Supplementary material for: Revisiting the Importance of Amplifying Bias for Debiasing
Source: arXiv:2205.14594 source file (2022-12-07)
Supplement: Supplementary file 1 [file supplementary.tex]

% %File: anonymous-submission-latex-2023.tex
% \documentclass[letterpaper]{article} % DO NOT CHANGE THIS
% \usepackage[submission]{aaai23}  % DO NOT CHANGE THIS
% \usepackage{times}  % DO NOT CHANGE THIS
% \usepackage{helvet}  % DO NOT CHANGE THIS
% \usepackage{courier}  % DO NOT CHANGE THIS
% \usepackage[hyphens]{url}  % DO NOT CHANGE THIS
% \usepackage{graphicx} % DO NOT CHANGE THIS
% \urlstyle{rm} % DO NOT CHANGE THIS
% \def\UrlFont{\rm}  % DO NOT CHANGE THIS
% \usepackage{natbib}  % DO NOT CHANGE THIS AND DO NOT ADD ANY OPTIONS TO IT
% \usepackage{caption} % DO NOT CHANGE THIS AND DO NOT ADD ANY OPTIONS TO IT
% \frenchspacing  % DO NOT CHANGE THIS
% \setlength{\pdfpagewidth}{8.5in} % DO NOT CHANGE THIS
% \setlength{\pdfpageheight}{11in} % DO NOT CHANGE THIS
% %
% % These are recommended to typeset algorithms but not required. See the subsubsection on algorithms. Remove them if you don't have algorithms in your paper.
% % \usepackage{algorithm}
% % \usepackage{algorithmic}
% \usepackage{algorithm}% http://ctan.org/pkg/algorithm
% \usepackage{algpseudocode}%
% \usepackage{fancyhdr}
% \usepackage[ruled,vlined]{algorithm2e}
% \usepackage{setspace}

% %%%%% Additional Packages (220515) %%%%%
% \usepackage{graphicx}
% \usepackage{booktabs}
% \usepackage{multirow}
% \usepackage{mathtools}

% \usepackage{pifont}% http://ctan.org/pkg/pifont
% \usepackage{pdfrender}
% \newcommand{\cmark}{\ding{51}}%   % 52
% \newcommand{\xmark}{\ding{55}}%
% \usepackage{colortbl}

% \usepackage{stfloats} % table

% \usepackage{cite}

% \newcommand{\stdv}[1]{\scriptsize$\pm$#1}

% \newcommand*{\boldcheckmark}{%
%   \textpdfrender{
%     TextRenderingMode=FillStroke,
%     LineWidth=.5pt, % half of the line width is outside the normal glyph
%   }{\cmark}%
% }
% \newcommand*{\boldxmark}{%
%   \textpdfrender{
%     TextRenderingMode=FillStroke,
%     LineWidth=.5pt, % half of the line width is outside the normal glyph
%   }{\xmark}%
% }

% \definecolor{Gray}{gray}{0.95}

% \definecolor{MyGreen}{rgb}{0,0.6,0.3}
% \definecolor{blackpink}{rgb}{0.6,0,0.6}
% \definecolor{MyRed}{RGB}{200, 0, 0}
% \newcommand{\dy}[1]{{\color{MyRed}#1}}
% \newcommand{\jh}[1]{{\color{MyGreen}#1}}
% \newcommand{\js}[1]{{\color{blackpink}#1}}

% %
% % These are are recommended to typeset listings but not required. See the subsubsection on listing. Remove this block if you don't have listings in your paper.
% \usepackage{newfloat}
% \usepackage{listings}
% \DeclareCaptionStyle{ruled}{labelfont=normalfont,labelsep=colon,strut=off} % DO NOT CHANGE THIS
% \lstset{%
% 	basicstyle={\footnotesize\ttfamily},% footnotesize acceptable for monospace
% 	numbers=left,numberstyle=\footnotesize,xleftmargin=2em,% show line numbers, remove this entire line if you don't want the numbers.
% 	aboveskip=0pt,belowskip=0pt,%
% 	showstringspaces=false,tabsize=2,breaklines=true}
% \floatstyle{ruled}
% \newfloat{listing}{tb}{lst}{}
% \floatname{listing}{Listing}
% %
% % Keep the \pdfinfo as shown here. There's no need
% % for you to add the /Title and /Author tags.
% \pdfinfo{
% /TemplateVersion (2023.1)
% }

% % DISALLOWED PACKAGES
% % \usepackage{authblk} -- This package is specifically forbidden
% % \usepackage{balance} -- This package is specifically forbidden
% % \usepackage{color (if used in text)
% % \usepackage{CJK} -- This package is specifically forbidden
% % \usepackage{float} -- This package is specifically forbidden
% % \usepackage{flushend} -- This package is specifically forbidden
% % \usepackage{fontenc} -- This package is specifically forbidden
% % \usepackage{fullpage} -- This package is specifically forbidden
% % \usepackage{geometry} -- This package is specifically forbidden
% % \usepackage{grffile} -- This package is specifically forbidden
% % \usepackage{hyperref} -- This package is specifically forbidden
% % \usepackage{navigator} -- This package is specifically forbidden
% % (or any other package that embeds links such as navigator or hyperref)
% % \indentfirst} -- This package is specifically forbidden
% % \layout} -- This package is specifically forbidden
% % \multicol} -- This package is specifically forbidden
% % \nameref} -- This package is specifically forbidden
% % \usepackage{savetrees} -- This package is specifically forbidden
% % \usepackage{setspace} -- This package is specifically forbidden
% % \usepackage{stfloats} -- This package is specifically forbidden
% % \usepackage{tabu} -- This package is specifically forbidden
% % \usepackage{titlesec} -- This package is specifically forbidden
% % \usepackage{tocbibind} -- This package is specifically forbidden
% % \usepackage{ulem} -- This package is specifically forbidden
% % \usepackage{wrapfig} -- This package is specifically forbidden
% % DISALLOWED COMMANDS
% % \nocopyright -- Your paper will not be published if you use this command
% % \addtolength -- This command may not be used
% % \balance -- This command may not be used
% % \baselinestretch -- Your paper will not be published if you use this command
% % \clearpage -- No page breaks of any kind may be used for the final version of your paper
% % \columnsep -- This command may not be used
% % \newpage -- No page breaks of any kind may be used for the final version of your paper
% % \pagebreak -- No page breaks of any kind may be used for the final version of your paperr
% % \pagestyle -- This command may not be used
% % \tiny -- This is not an acceptable font size.
% % \vspace{- -- No negative value may be used in proximity of a caption, figure, table, section, subsection, subsubsection, or reference
% % \vskip{- -- No negative value may be used to alter spacing above or below a caption, figure, table, section, subsection, subsubsection, or reference

% \setcounter{secnumdepth}{0} %May be changed to 1 or 2 if section numbers are desired.

% % The file aaai23.sty is the style file for AAAI Press
% % proceedings, working notes, and technical reports.
% %

% % Title

% % Your title must be in mixed case, not sentence case.
% % That means all verbs (including short verbs like be, is, using,and go),
% % nouns, adverbs, adjectives should be capitalized, including both words in hyphenated terms, while
% % articles, conjunctions, and prepositions are lower case unless they
% % directly follow a colon or long dash
% \title{Supplementary for \\Revisiting the Importance of Amplifying Bias for Debiasing}
% \author{
%     %Authors
%     % All authors must be in the same font size and format.
%     Written by AAAI Press Staff\textsuperscript{\rm 1}\thanks{With help from the AAAI Publications Committee.}\\
%     AAAI Style Contributions by Pater Patel Schneider,
%     Sunil Issar,\\
%     J. Scott Penberthy,
%     George Ferguson,
%     Hans Guesgen,
%     Francisco Cruz\equalcontrib,
%     Marc Pujol-Gonzalez\equalcontrib
% }
% \affiliations{
%     %Afiliations
%     \textsuperscript{\rm 1}Association for the Advancement of Artificial Intelligence\\
%     % If you have multiple authors and multiple affiliations
%     % use superscripts in text and roman font to identify them.
%     % For example,

%     % Sunil Issar, \textsuperscript{\rm 2}
%     % J. Scott Penberthy, \textsuperscript{\rm 3}
%     % George Ferguson,\textsuperscript{\rm 4}
%     % Hans Guesgen, \textsuperscript{\rm 5}.
%     % Note that the comma should be placed BEFORE the superscript for optimum readability

%     1900 Embarcadero Road, Suite 101\\
%     Palo Alto, California 94303-3310 USA\\
%     % email address must be in roman text type, not monospace or sans serif
%     publications23@aaai.org
% %
% % See more examples next
% }

% %Example, Single Author, ->> remove \iffalse,\fi and place them surrounding AAAI title to use it
% \iffalse
% \title{My Publication Title --- Single Author}
% \author {
%     Author Name
% }
% \affiliations{
%     Affiliation\\
%     Affiliation Line 2\\
%     name@example.com
% }
% \fi

% \iffalse
% %Example, Multiple Authors, ->> remove \iffalse,\fi and place them surrounding AAAI title to use it
% \title{My Publication Title --- Multiple Authors}
% \author {
%     % Authors
%     First Author Name,\textsuperscript{\rm 1}
%     Second Author Name, \textsuperscript{\rm 2}
%     Third Author Name \textsuperscript{\rm 1}
% }
% \affiliations {
%     % Affiliations
%     \textsuperscript{\rm 1} Affiliation 1\\
%     \textsuperscript{\rm 2} Affiliation 2\\
%     firstAuthor@affiliation1.com, secondAuthor@affilation2.com, thirdAuthor@affiliation1.com
% }
% \fi


% % REMOVE THIS: bibentry
% % This is only needed to show inline citations in the guidelines document. You should not need it and can safely delete it.
% \usepackage{bibentry}
% % END REMOVE bibentry

% \begin{document}

% \maketitle

% \appendix
% % \section{Supplementary Material}
% % This supplementary presents the following: 1) additional GradCAM~\cite{gradcam} visualizations of multiple $f_{B}^*$ capturing diverse visual attributes, 2) how our data sample selection method further amplifies bias when training $f_B$, 3) stable performance of using multiple BCDs, 4) the comparisons of debiasing performance on the unbiased test sets with the standard deviation, 5) the pseudo-code of our training procedure, 6) performance degradation of our method with strict agreement votes, 7) detailed descriptions of datasets, 8) further implementation details, and 9) the limitation of our work. 
% % Our codes and datasets are available at \url{https://tinyurl.com/neurips2022-4847}.\footnote{We are planning to release them on GitHub after our paper is accepted.}


% This supplementary presents additional experiments and further explanations of our approach that we could not include in the main paper due to the page limit. 
% Our codes and datasets are available at \url{https://tinyurl.com/aaai2023-2679}.\footnote{We are planning to release them on GitHub after our paper is accepted.}

% \section{Comparisons with Ensembles}
% \input{tables/supp_ens}
% \subsection{Ensembling $f_B$}
% As mentioned in the main paper, our proposed method is different from simply ensembling multiple biased models. 
% We conducted experiments to demonstrate that our proposed method is superior to simply ensembling multiple biased models.
% For the experiment, we jointly trained $f_D$ with multiple biased models ($f_{B_1}$, $f_{B_2}$, ... $f_{B_5}$) during the main stage of debiasing. 
% Note that $f_{B_i}$ are biased models which are jointly trained with $f_D$ for computing reweighting value $w$, not the pretrained biased models which are denoted as $f^*_{B_i}$ used to filter bias-conflicting samples in our method.
% For the reweighting value $w$, we computed the Cross Entropy loss with the averaged softmax probabilities of the five $f_{B_i}$ models which is formulated as 
% \begin{equation}
%         w(x) = \frac{\mathcal{L_\text{CE}}(\frac{1}{M}\sum^{M}_{i=1} f_{B_i}(x), y)}{\mathcal{L_\text{CE}}(\frac{1}{M}\sum^{M}_{i=1} f_{B_i}(x), y) + \mathcal{L_\text{CE}}(f_D(x), y)}
% \end{equation}
% where $M$ is set to 5.

% Table~\ref{tab:supp_ensemble} shows that our proposed method is superior to ensembling multiple biased models in the main stage of debiasing. 
% The main reason is that the bias-conflicting samples are not discarded when training them, so each biased model $f_{B_i}$ gradually learns the intrinsic attribute as training proceeds.
% % Since the bias-conflicting samples do not have bias attributes while including the intrinsic attributes, each biased model $f_{B_i}$ gradually learn the intrinsic attribute as training proceeds. 
% Fig.~\ref{fig:supple-ensemble-graph} supports the point.
% Fig.~\ref{fig:supple-ensemble-graph} visualizes each metric used in Fig.~2 of the main paper.
% We report the averaged values of $f_{B_i}$ for the accuracies of $f_B$ on the unbiased test set and biased test set. 
% We observe that the average accuracy of $f_{B_i}$ models on the unbiased test set increases as training steps proceed even with ensembling them. 
% % ensemble은 원래 task에서 잘하는건데 하나라도 conflicting을 맞추면 성능 하락 

% \subsection{Ensembling $f_D$}
% One might also question the effectiveness of ensembling $f_D$ in the main stage of debiasing. 
% We want to clarify that the main contribution of our paper is revealing that amplifying bias via utilizing predictions of multiple pretrained \emph{biased} models is crucial for improving debiasing performance.
% In other words, ensembling multiple \emph{debiased} models is orthogonal to our work. 
% % Unlike ensembling biased models, ensemble of multiple debiased models can be easily done without careful consideration because the target labels are explicitly provided.
% In Table~\ref{tab:supp_ensemble}, we also ensemble multiple debiased models of LfF.
% % In Table~\ref{tab:supp_ensemble}, we observe that ensembling multiple debiased models in LfF brings performance gain compared to the original training of LfF.
% We observe that ensembling multiple debiased models in LfF brings performance gain compared to the original training of LfF.
% However, applying our sample selection method to LfF without ensembling multiple debiased models still shows superior performance to ensembling multiple debiased models of LfF.
% Note that ensembling of debiased models requires large computational cost and memory space for inference, unlike our proposed method.


% % Ensembling has been widely adopted in machine learning and deep learning, showing consistent performance boost. 
% % However, this experiment shows that ensembling without careful consideration does not guarantee performance gain in debiasing. 
% % While ensembling itself may be regarded as a simple and naive approach, we believe that finding how to adjust ensembling to debiasing task is an important issue and needs careful consideration.
% % Based on the finding, we proposed a simple yet effective data sample selection which only requires a minimal amount of additional training steps. 


% % We revealed that a bias attribute may form of multiple visual attributes and utilizing multiple pretrained biased models enables to capture the bias attribute comprehensively in the main paper. 

% \begin{figure*}[t]
%     \centering
%     % \includegraphics[width=0.85\textwidth]{figures/fig_lff_vs_ours_aligned.pdf}
%     \includegraphics[width=0.85\textwidth]{figures/fig_lffwEns_vs_ours.pdf}
%     \caption{
%     Comparison of LfF 1) with ensembling multiple $f_B$ models (blue) and 2) with our method (red). (a) and (b) indicate the results on Colored MNIST and BFFHQ, respectively. Each metric corresponds to the ones used in Fig. 2 of the main paper. For column 1 and column 2, we averaged the values of multiple $f_{B_i}$ for reporting the case of ensembling multiple $f_{B_i}$.
%     }
%     \vspace{0.1cm}
%     \label{fig:supple-ensemble-graph}
% \end{figure*}



% \begin{figure*}[h!]
%     \centering
%     \includegraphics[width=0.7\linewidth]{figures/bias_heatmap_big_2.pdf}
%     \caption{Recall values of overlapped regions between the highlighted pixels and the segmentation map of each facial attribute. The values are different among each $f_{B_i}$, indicating that differently initialized models focus on different facial attributes.}
%     % \vspace{-0.1cm}
%     \label{fig:gradcam_heatmap}
% \end{figure*}


% \begin{figure*}[h!]
%     \centering
%     \includegraphics[width=1.0\textwidth]{figures/supplementary_gradcam_v3.pdf}
%     \caption{Additional results of GradCAM on each $f_{B}^*$. The first column indicates the original images. Starting from the second column, we visualize GradCAM using each biased model~(\textit{i.e.,} $f_{B_1}^*,\dots,f_{B_5}^*$).}
%     \vspace{-0.25cm}
%     \label{fig:supple-gradcam}
% \end{figure*}

% \input{tables/supp_time_params}
% \input{tables/supp_f_B}
% \input{tables/supp_55K}

% % \section{Visualization of Multiple $f_{B}^*$ Capturing Diverse Visual Attributes}
% \section{Multiple $f_{B}^*$ Capturing Diverse Visual Attributes}
% \label{supple:gradcam}
% In the main paper, we showed the results of GradCAM visualization of each $f_{B}^*$ which demonstrate that each biased model utilizes different facial attributes for making biased predictions. 
% This section supports such a fact by showing the quantitative measurement of how each biased model focuses on different parts of images. 
% By using the GradCAM visualization of each image, we obtained pixels of an image whose the values of GradCAM are higher than a certain threshold.
% We name such pixels as `highlighted pixels'.
% Since the scale of GradCAM is between 0 to 1, we chose the threshold as 0.5.
% Then, we utilized a segmentation mask~\cite{or2020lifespan} of FFHQ~\cite{stylegan} including semantic classes such as eyes, lips, hair, and so on.
% We compute the recall value, $S$, of the overlapped region between the highlighted pixels and the segmentation map of each facial attribute which can be formulated as, 
% \begin{equation}
%     S = \frac{A_{overlap}}{A_{mask}}
% \end{equation}
% where $A_{overlap}$ and $A_{mask}$ indicate the area of the overlapped region and that of the segmentation mask of each facial attribute, respectively. 
% In Fig.~\ref{fig:gradcam_heatmap}, we observe that $S$ values of the facial attributes are different in each $f_{B_i}^*$.
% For example, $S$ values of lip and mouth are high for $f_{B_1}^*$ while those of eye and eyebrows are high for $f_{B_5}^*$. 
% This again demonstrates that differently initialized biased models focus on different visual attributes. 
% Note that among 19 facial attributes in the segmentation mask dataset, we selectively chose the ones which may contribute to making biased predictions towards gender.
% While ears and neck may not contribute to predicting the gender, they are located near to the facial attributes which may contribute to making biased predictions (\textit{e.g.,} ears are close to hair and neck is close to the lip).
% Thus, we included such visual attributes in our analysis. 

% As done in the main paper, we show additional results of GradCAM visualization in Fig.~\ref{fig:supple-gradcam}. 
% We again observe that each $f_{B}^*$ focuses on different part of image for making biased predictions. 
% % We visualize how each $f_{B}^*$ captures the bias attribute by using GradCAM~\cite{gradcam} in Fig.~\ref{fig:gradcam} in order to demonstrate that biased models $f_{B}^*$ with different random initialization focus on different visual attributes.
% % For the visualization, we use BFFHQ of which the intrinsic attribute and the bias attribute are the age and the gender, respectively.
% % We show images which all five $f^{*}_B$ predict with the correct bias labels in Fig.~\ref{fig:gradcam}.
% % The first column indicates the original images while the other columns indicate the GradCAM of each $f^{*}_B$, respectively. 
% % We observe that each $f^{*}_B$ focuses on different visual attributes. 
% % For example, $f_{B_1}^*$ focuses on the mouth for predicting the gender (\textit{e.g.,} focusing on lip makeups for females and mustaches for males). 
% % On the other hand, $f_{B_3}^*$ and $f_{B_4}^*$ heavily rely on the hair for predicting the gender. 
% % Meanwhile, $f_{B_2}^*$ and $f_{B_5}^*$ uses the nose and eyes for making predictions. 

% % As mentioned in the main paper, a bias (\textit{e.g.,} gender) can be formed in a combination of multiple visual attributes (\textit{e.g.,} hair, mustache, eyes, makeup, etc). 
% % However, in Fig.~\ref{fig:gradcam}, we observe that each biased model only uses a certain visual cue (\textit{e.g.,} mustache or hair) for making predictions, partially capturing the bias attribute.
% % Utilizing multiple BCDs in our method mitigates such an issue since it regards an image as a bias-aligned one only if the image includes at least half number of visual attributes contributing the model to be biased. 
% % Such visualization demonstrates the necessity of ensembling multiple biased models compared to using a single one.  


% % \clearpage




% % Computational Costs -> training step으로 바꿔봤어 Computational costs가 둘다를 포함하는거 같아서
% \section{Analysis on Training Steps and Memory Space}
% % This section analyzes the training time and memory space of our proposed method.

% \noindent\textbf{Training Steps. \enskip}
% We compare the number of iterations for training models with and without our approach in Table~\ref{table:supp_time_params}.
% Since we train each biased model $f_B^*$ with a small number of iterations (1K), the additional computational cost of our approach is marginal.  
% % jh
% % It only takes 5K iterations for training our data selection module when iteratively training the five biased models.
% Our data selection module only necessitates additional 5K iterations while iteratively pretraining the five biased models. 
% Also, Table~\ref{table:supp_55k} demonstrates that simply using additional 5K training steps on existing reweighting-based debiasing approaches does not bring performance gain. 
% In other words, it is necessary to utilize additional small number of training steps in an adequate manner. 

% \noindent\textbf{Memory Space. \enskip}
% Generally, ensemble methods need multiple model checkpoints to be stored in memory to make multiple predictions at the \emph{inference time}.
% However, unlike such ensemble methods, our approach only needs to assign pseudo labels on the \emph{training samples}, so we do not have to save the model checkpoints for the purpose of using them at the \emph{test phase}.
% Without saving the multiple model checkpoints in the memory space, we obtain the predictions of a biased model on the training samples, and re-initialize the next biased model with the same memory.
% Table~\ref{table:supp_time_params} demonstrates that our method does not require additional number of parameters for the existing reweighting-based debiasing methods. 
% % For the memory space, we report the maximum number of parameters required to be saved in the memory in the Table~\ref{table:supp_time_params}.
% % The results demonstrate that our data selection module does not require any additional memory space.
% We explain the detailed procedure with a pseudo code in the section named "Pseudo-code of Our Training Procedure" in this Supplementary regarding such an issue.
% % To obtain the predictions from multiple biased models, we can train a model and forward the training samples, iteratively. 
% % Specifically, without saving the multiple model \js{checkpoints} in the memory, the model parameters can be re-initialized to train the following model after acquiring the predictions. (See section named "Pseudo-code of Our Training Procedure" in Supplementary.)

% \section{Amplified Bias via Bias Amplified Dataset}
% % \section{Amplified Bias via Bias Sample Selection}
% \label{supple:amplified-bias}

% % \noindent \textbf{}
% Table~\ref{tab:supple_bias_unbiased} shows the image classification accuracy of $f_B$ on the biased and unbiased test set. 
% % We compare LfF~\cite{nam2020learning} without BE and LfF with BE using the test set accuracy at the last epoch in Table~\ref{tab:supple_bias_unbiased}. 
% We compare LfF~\cite{nam2020learning} 1) without our method and 2) with our method using the test set accuracy at the last epoch in Table~\ref{tab:supple_bias_unbiased}. 
% As mentioned in the main paper, a biased model achieves 1) low accuracy on the unbiased test set and 2) high accuracy on the biased test set.
% In other words, the difference between the accuracy of the biased test set and that of the unbiased test set, $\text{acc}_{\text{diff}}$ in Table~\ref{tab:supple_bias_unbiased}, is high for the biased models.
% This is due to the fact that the biased model heavily relies on the bias attributes while failing to learn the intrinsic attributes. 

% As shown in Table~\ref{tab:supple_bias_unbiased}, using our biased sample selection module significantly increases the $\text{acc}_{\text{diff}}$ indicating that utilizing our method further amplifies bias for $f_B$. 
% To be more specific, applying our method achieves low unbiased test set accuracy and high biased test set accuracy in Colored MNIST.
% Meanwhile, we observe a minimal performance drop in the biased test set with other datasets.
% However, considering the significant performance drop on the unbiased test set and high $\text{acc}_{\text{diff}}$, such a drop in biased test set accuracy is negligible.
% The result shows that the debiasing performance gain of our method is due to the amplified bias of $f_B$.
% It again demonstrates the fact that two factors are crucial for amplifying bias: 1) improving the biased test set accuracy of $f_B$ and 2) degrading the unbiased test set accuracy of $f_B$ (\textit{i.e.,} not learning intrinsic attributes). 



% \begin{figure*}[h!]
%     \centering
%     \includegraphics[width=0.9\linewidth]{figures/ens_ablation_v2.pdf}
%     \vspace{-0.2cm}
%     \caption{
%     Comparison of models trained with 1) a single BCD ($M=1$, blue) and 2) multiple BCDs ($M=5$, red) on Dogs \& Cats. 
%     The shaded areas show the variations of the results on five different independent trials.
%     Each metric corresponds to the ones used in Fig.~2 of the main paper.}
%     \vspace{-0.6cm}
%     \label{fig:ens_ablation}
% \end{figure*}
% \input{tables/ablation_num_voting_five}


% % \section{Stable Performance of Using Multiple BCDs}
% \section{Performance Variation of Single/Multiple BCDs}
% \label{supple:stable-multiple}
% % As mentioned in Section~5.3 of the main paper, 
% As mentioned in the main paper, utilizing multiple BCDs reduces the performance variations compared to using a single BCD.
% Fig.~\ref{fig:ens_ablation} demonstrates the fact by visualizing the metrics used in Fig.~2 of the main paper with Dogs \& Cats dataset. 
% The shaded regions indicate the performance variation, the differences between five independent trials on a given metric. 
% We observe that utilizing multiple BCDs (red) shows smaller variations in terms of $w(x)$ of bias-conflicting samples and the unbiased test set accuracy of $f_D$.
% Again, this is due to the fact that leveraging multiple numbers of $f_B^{*}$ enables to consider multiple visual attributes, better capturing and understanding the bias attribute compared to using a single $f_B^{*}$.


% \section{Biased Sample Selection with Strict Agreements}
% \label{supple:be-strict}

% % As mentioned in Section~5.3 of the main paper, two factors are crucial for constructing a bias-amplified dataset $\mathcal{D}_A$: 1) discarding a sufficient number of bias-conflicting samples and 2) maintaining a reasonable number of bias-aligned ones. 
% There are two factors crucial for constructing a bias-amplified dataset $\mathcal{D}_A$: 1) discarding a sufficient number of bias-conflicting samples and 2) maintaining a reasonable number of bias-aligned ones. 
% We further demonstrate such a point by designing a strict version of the sample selection module in Table~\ref{tab:ablation_voting_five}; we regard a sample as a bias-conflicting one only if all five BCDs consider it as a bias-conflicting sample.
% $\mathcal{N}_{a}$ in Table~\ref{tab:ablation_voting_five} indicates the number of agreement votes required for deciding a sample as a bias-conflicting one. 
% We add our sample selection method on LfF~\cite{nam2020learning} with $\mathcal{N}_{a}$ set to three and five, and compare them with the original LfF. 
% Note that the number of BCDs, $M$, is fixed to five.

% Utilizing our biased sample selection method with $\mathcal{N}_{a}$=5 outperforms the original LfF.
% However, we observe that utilizing the selection method with $\mathcal{N}_{a}$=3 is superior to the method with $\mathcal{N}_{a}$=5. 
% The main reason is due to the number of bias-aligned and bias-conflicting samples. 
% Similar to Table~4 of the main paper, we report the remaining samples of bias-aligned samples and bias-conflicting samples in $\mathcal{D}_A$ by showing the adjusted ratio compared to each group in $\mathcal{D}$.
% We observe that utilizing our method with $\mathcal{N}_{a}$=5 discards the bias-conflicting ones significantly while also filtering out a considerable number of the bias-aligned ones.
% For example, by utilizing $\mathcal{N}_{a}$=5 in BFFHQ, there exist only 2.29\% of bias-conflicting samples in $\mathcal{D}_A$ compared to $\mathcal{D}$.
% However, only 57.48\% of bias-aligned samples are remained in $\mathcal{D}_A$, limiting $f_B$ to be further biased. 
% % \newpage


% \input{tables/supp_JTT}
% \section{Applicability of our method}
% We demonstrated the effectiveness of our proposed method on existing reweighting-based state-of-the-art debiasing methods~\cite{nam2020learning, disentangled}. 
% This section describes how our method can be applied to other debiasing methods. 
% Liu~\textit{et al.}~\shortcite{jtt} proposed JTT which 1) identifies misclassified samples, those regarded as bias-conflicting ones, in the first stage and 2) emphasizes those when training a debiased classifier in the second stage. 
% % In JTT, the authors train a biased classifier using the original Cross Entropy in the first stage. 
% We modified the first-stage training with our biased sample selection method. 
% We observe that our method brings large debiasing performance gain in JTT. 
% Such a result demonstrates that our method can be applied not only to reweighting-based methods but also to debiasing methods which need to identify bias-conflicting samples.
% % Such a result shows the applicability of our method beyond the reweighting-based debiasing methods. 
% % \label{supple:discussion}

% \input{tables/supp_CE_GCE}
% % \section{Analysis on the training loss for $f^*_B$}
% \vspace{-0.2cm}
% \section{Training $f^*_B$ with CE vs GCE}
% % \label{supple:CE_GCE}
% As mentioned in the main paper, we pretrain multiple $f^*_{B_i}$ for a small number of iterations by using the property that the bias is easy to learn. 
% Although the bias attribute is relatively easy to learn compared to the intrinsic attribute, we need to utilize the GCE loss rather than the CE loss. 
% We compared the debiasing performance between using CE loss and GCE loss for pretraining multiple $f^*_{B_i}$ in our method. 
% We observe that training multiple $f^*_{B_i}$ with GCE loss is superior to training it with CE loss.
% % Although the bias attribute is easy to learn, we need to utilize a loss function such as GCE loss which emphasizes the easy-to-learn samples (\textit{i.e.,} bias-aligned samples) rather than the original CE loss to further amplify bias.
% This is because GCE loss further amplifies bias compared to the original CE loss by emphasizing the easy-to-learn samples (\textit{i.e.,} bias-aligned samples).
% GCE loss has been widely used in the previous debiasing studies~\cite{nam2020learning,disentangled} for emphasizing bias-aligned samples, resulting a model to be overfitted to a bias overall. 

% \vspace{-0.25cm}
% \section{Further Implementation Details}
% \label{supple:implementation}
% \noindent \textbf{Experimental settings. \enskip}
% We set the learning rate as 0.01, 0.0001, 0.0001, and 0.00001 for Colored MNIST, BFFHQ, Dogs \& Cats, and BAR, respectively. 
% The image sizes are 28$\times$28 for Colored MNIST and 224$\times$224 for the rest of the datasets. 
% For Colored MNIST, we do not apply additional data augmentation techniques.
% For BFFHQ, Dogs \& Cats, and BAR, we apply random crop and horizontal flip transformations. 
% Also, images are normalized along each channel (3, H, W) with the mean of (0.4914, 0.4822, 0.4465) and standard deviation of (0.2023, 0.1994, 0.2010). 
% We conducted all experiments using a single V100 GPU. 
% % \jh{Other hyperparameters specialized for each baselines are following its original paper.}
% We used the default values of hyperparameters reported in the original paper for the baseline models.
% Applying our method on LfF~\cite{nam2020learning} requires approximately up to 0.8GB of memory for Colored MNIST and 4.3GB of memory for the rest of the datasets.
% \newline 

% \noindent \textbf{Applying Our Method on Reweighting-based Methods.\enskip}
% As aforementioned in the main paper, when applying our method to the existing reweighting-based approaches (\textit{i.e.,} LfF~\cite{nam2020learning} and DisEnt~\cite{disentangled}), we do not modify the training procedure of the debiased model $f_{D}$.
% For both methods, we train $f_{B}$ using the bias-amplified dataset $\mathcal{D}_A$.
% DisEnt, unlike LfF, additionally utilizes feature-level data augmentation during training.
% When we apply our selection method to DisEnt, we use $\mathcal{D}_A$ for training the parameters which are updated with respect to the feature vectors of bias attributes.
% $f_B$ of our paper corresponds to $E_b$ and $C_b$ in the original paper of DisEnt~\cite{disentangled}.


% \begin{figure*}[t!]
%     \centering
%     \includegraphics[width=0.85\linewidth]{figures/sup_dataset.pdf}
%     \vspace{+0.5cm}
%     \caption{Illustrative example of the datasets used in our work.
%     Each column in Colored MNIST and BAR dataset indicates each class, while the group of three columns in BFFHQ and Dogs \& Cats indicate each class. The images above the dotted line are the bias-aligned samples, while the ones below indicate the bias-conflicting samples. 
%     % For better understanding, we present a bigger figure of datasets compared to the one in the main paper.
%     }
%     \vspace{+1cm}
%     \label{fig:supple-dataset}
% \end{figure*}

% \input{tables/supp_ablation_align_conflict}
% \input{tables/supp_ablation_threshold}

% % \newpage

% \section{Additional Experimental Results}
% % \label{supple:discussion}
% We additionally report the results which we intentionally omitted in the main paper due to the page limit. 
% Table~\ref{tab:supp_ablation_align_conflict} shows the tendency of debiasing performance with additional cases of adjusted numbers of bias-aligned and bias-conflicting samples (Table~2 of the main paper). 
% We also included the standard deviation of each result. 
% Table~\ref{tab:supp_ablation_threshold} includes the standard deviations of results demonstrating the robustness of our proposed method to a wide range of confidence threshold $\tau$ (Table~5 of the main paper).

% \vspace{-0.1cm}
% \section{Further Details on Datasets}
% \label{supple:dataset}
% Fig.~\ref{fig:supple-dataset} shows the dataset used in our work.

% \noindent \textbf{Colored MNIST. \enskip} 
% We modify MNIST dataset~\cite{mnist} and set the color as the bias attribute. 
% Each one of the ten digits is highly correlated with a certain color (\textit{e.g.,} red for 0). We inject the color into the foreground of each image. 
% For Colored MNIST, we conduct experiments with the dataset used in Lee~\textit{et al.}~\shortcite{disentangled}.
% For each ratio of bias-conflicting samples, the number of bias-aligned samples and bias-conflicting samples are as follows: ($54751$, $249$)-$0.5\%$, ($54509$, $491$)-$1\%$, ($54014$, $986$)-$2\%$, and ($52551$, $2449$)-$5\%$.

% \newline

% \noindent \textbf{BFFHQ. \enskip} 
% We used BFFHQ which was first introduced in Kim~\textit{et al.}~\shortcite{biaswap}. 
% BFFHQ sets the age (\textit{i.e.,} old and young) as the intrinsic attribute and the gender as the bias attribute. 
% Bias-aligned samples are young (\textit{i.e.,} age ranging from 10 to 29) females and old (\textit{i.e.,} age ranging from 40 to 59) males. 
% For each ratio of bias-conflicting sample, the number of bias-aligned samples and bias-conflicting samples are as follows: ($19104$, $96$)-$0.5\%$, ($19008$, $192$)-$1\%$, ($18816$, $384$)-$2\%$, and ($18240$, $960$)-$5\%$.
% Following the work of Lee~\textit{et al.}~\shortcite{disentangled}, we exclude the bias-aligned samples from the unbiased test set since it only includes two target classes.

% \newline

% \noindent \textbf{Dogs \& Cats. \enskip}
% Dogs \& Cats~\footnote{\url{https://www.kaggle.com/c/dogs-vs-cats-redux-kernels-edition}} was first used in Kim et al.~\shortcite{LNL}.
% However, we find that the test sets used in the work do not have publicly available ground truths. 
% Therefore, since the original train set has ground truth labels, we split the original train set into train, valid, and test sets.
% For each ratio of bias-conflicting sample, the number of bias-aligned samples and bias-conflicting samples are as follows: ($8037$, $80$)-$1\%$ and ($8037$, $452$)-$5\%$.
% We did not include the bias-aligned samples in the unbiased test set. 

% \noindent \textbf{BAR. \enskip} 
% In the work of Nam~\textit{et al.}~\shortcite{nam2020learning}, the original BAR dataset does not include bias-conflicting samples in the training set.
% However, for the consistent experimental setting and for the evaluation under various bias severities, we build two sets of BAR dataset with different ratios of bias-conflicting samples. 
% For each ratio of bias-conflicting sample, the number of bias-aligned samples and bias-conflicting samples are as follows: ($1761$, $14$)-$1\%$ and ($1761$, $85$)-$5\%$.
% We did not include the bias-aligned samples in the unbiased test set. 




% \input{tables/supp_main_bast_test_1}
% \input{tables/supp_main_best_test_2}

% \begin{figure*}[h]
% \centering
% \begin{minipage}{\textwidth}
% \begin{algorithm}[H]
% \caption{Biased sample selection module added to reweighting-based debiasing methods}
% \setstretch{1.3}
% \SetAlgoLined
% \KwIn{iteration for pretraining $t_B$, dataset $\mathcal{D}$, confidence threshold $\tau$, the number of biased models used in our sample selection module $M$}

% % Initialize biased models ${f_{B_1}^*, \dots, f_{B_M}^*}$ \Comment{Pretrain biased models} \\

% Initialize network $f_B$\\
% \For{$i = 1, 2, ..., M$}{
% Re-initialize the network $f_B$ with randomized parameters $\theta_i^*$ to train a biased model $f_{B_i}^*$ \Comment{Pretrain biased models}\\
% \For{$t = 1, 2, ..., t_B$} 
% {Update ${\theta_{i}^*}$ using $\mathcal{D}$ with $\mathcal{L}_\text{GCE}$}
% % {Update ${f_{B_i}^*}$ using $\mathcal{D}$ with $\mathcal{L}_\text{GCE}$}
% $f_{B_i}^* \gets f_B \text{ parameterized with } {\theta_{i}^*}$ \\
% \For{$(x, y) \in \mathcal{D}$}{
% Calculate and save the value of $p_y(x; f_{B_i}^*)$
% }
% }


% $\mathcal{D}_A \gets \emptyset $  \Comment{Construct the bias-amplified dataset $\mathcal{D}_A$}\\ 
% % Build $M$ bias-conflicting detectors ($BCD$s) with ${f_{B_1}^*, \dots, f_{B_M}^*}$ \\
% \For{$(x, y) \in \mathcal{D}$}{
% %%%% 원래 %%%%
% % \For{$f \in \left\{f_{B_1}^*, \dots, f_{B_M}^*\right\}$}{ 
% %%%%%%%%%%%%
% \For{$i = 1, 2, ..., M$}{ 
% % \lIf{$p_y(x; f) < \tau$}{$BCD(x; \tau, f) \gets 0$}
% % \lElse{$BCD(x; \tau, f)\gets 1$}
% \eIf{$p_y(x; f_{B_i}^*) < \tau$}{$BCD(x; \tau, f_{B_i}^*)\gets 0$}{$BCD(x; \tau, f_{B_i}^*)\gets 1$}
% }
% }
% \If{$\sum_{i=1}^M{BCD(x; \tau, f_{B_i}^*)} \ge \lceil{\frac{M}{2}}\rceil$}{
%     $\mathcal{D}_A \gets \mathcal{D}_A \cup \left\{ (x, y) \right\}$ 
%     }

% Re-initialize $f_B$ and initialize $f_D$ \Comment{Train a debiased model}\\
% \While{\textit{not converged}}{
%     \For{$(x, y) \in \mathcal{D}$}{
%       Compute reweighting value $w(x)$ using $f_B$ and $f_D$ \par
%     %   \begin{varwidth}{\linewidth}
%         \If{$(x, y) \in \mathcal{D}_A$}{
%         Update $f_B$ using $\mathcal{D}_A$ with $\mathcal{L}_\text{CE}(f_B(x), y)$ }
%         Update $f_D$ using $\mathcal{D}$ with  $w(x)\cdot\mathcal{L}_\text{CE}(f_D(x), y)$ 
%     %   \end{varwidth}
%       }
% }

% \label{algorithm}
% \end{algorithm}
% \end{minipage}
% % \vspace{-0.3cm}
% \end{figure*}

% \vspace{-0.2cm}
% \section{Limitation}
% \label{supple:discussion}

% One limitation of our work is that there still exist a small number of bias-conflicting samples in $\mathcal{D}_A$ after applying our method.
% Ideally, a model trained with bias-aligned samples only would be perfectly biased towards the bias attribute.
% Since we do not use explicit bias labels, we could not discard all bias-conflicting samples when constructing $\mathcal{D}_A$ for training $f_B$.
% In the meanwhile, we filtered out a sufficient number of bias-conflicting samples, improving the debiasing performance of $f_D$ which has been demonstrated throughout the paper.

% \section{Comparisons of Debiasing Performance on Unbiased Test Sets}
% \label{supple:comparison-total-table}
% Due to the page limit, we intentionally omitted the standard deviation in Table~1 of the main paper. 
% Therefore, we present the quantitative results on the unbiased test sets including the standard deviations in Table~\ref{tab:supp_best_test_v1} and Table~\ref{tab:supp_best_test_v2}. 
% Note that the results are averaged over five individual trials. 

% \newpage
% \section{Pseudo-code of Our Training Procedure}
% \label{supple:pseudo-code}
% For a better understanding of the proposed sample selection method, we describe the training procedure of utilizing our method on existing reweighting-based debiasing methods using a pseudo-code. 
% % \clearpage

% % Use \bibliography{yourbibfile} instead or the References section will not appear in your paper
% % \nobibliography{aaai23}
% \clearpage
% \bibliography{aaai23}

% % \section{Acknowledgments}
% % AAAI is especially grateful to Peter Patel Schneider for his work in implementing the original aaai.sty file, liberally using the ideas of other style hackers, including Barbara Beeton. We also acknowledge with thanks the work of George Ferguson for his guide to using the style and BibTeX files --- which has been incorporated into this document --- and Hans Guesgen, who provided several timely modifications, as well as the many others who have, from time to time, sent in suggestions on improvements to the AAAI style. We are especially grateful to Francisco Cruz, Marc Pujol-Gonzalez, and Mico Loretan for the improvements to the Bib\TeX{} and \LaTeX{} files made in 2020.

% % The preparation of the \LaTeX{} and Bib\TeX{} files that implement these instructions was supported by Schlumberger Palo Alto Research, AT\&T Bell Laboratories, Morgan Kaufmann Publishers, The Live Oak Press, LLC, and AAAI Press. Bibliography style changes were added by Sunil Issar. \verb+\+pubnote was added by J. Scott Penberthy. George Ferguson added support for printing the AAAI copyright slug. Additional changes to aaai23.sty and aaai23.bst have been made by Francisco Cruz, Marc Pujol-Gonzalez, and Mico Loretan.

% \end{document}
