# Supplementary material for: Revisiting the Importance of Amplifying Bias for Debiasing
Source: arXiv:2205.14594 source file (2022-12-07)
Supplement: Supplementary file 2 [file appendix_best_test_acc.tex]

\begin{table}
\begin{center}
\scalebox{0.57}{
\begin{tabular}{ccccccccccc|ccc}
% \hline\noalign{\smallskip}
\toprule 
\multirow{2.5}{*}{Dataset} 
& \multirow{2.5}{*}{Ratio (\%)} 
&
& Vanilla~\cite{He2015resnet}
& HEX~\cite{wang2018hex}
& LNL~\cite{LNL}
& EnD~\cite{EnD}
& ReBias~\cite{bahng2019rebias}
& LfF~\cite{nam2020learning}
& DisEnt~\cite{disentangled}
& SoftCon~\cite{softcon}
& LfF + BE
& DisEnt + BE 
& Softcon + BE
\\
\cmidrule{4-14}
&&
& \textcolor{black}{\boldxmark} \textcolor{black}{\boldxmark}
& \textcolor{black}{\boldxmark} \textcolor{black}{\boldcheckmark}
& \textcolor{black}{\boldcheckmark} \textcolor{black}{\boldcheckmark}
& \textcolor{black}{\boldcheckmark} \textcolor{black}{\boldcheckmark}
& \textcolor{black}{\boldxmark} \textcolor{black}{\boldcheckmark}
& \textcolor{black}{\boldxmark} \textcolor{black}{\boldxmark}
& \textcolor{black}{\boldxmark} \textcolor{black}{\boldxmark}
& \textcolor{black}{\boldxmark} \textcolor{black}{\boldxmark}
& \textcolor{black}{\boldxmark} \textcolor{black}{\boldxmark}
& \textcolor{black}{\boldxmark} \textcolor{black}{\boldxmark}
& \textcolor{black}{\boldxmark} \textcolor{black}{\boldxmark}
\\
\midrule
\multirow{4}{*}{\makecell{Colored MNIST}} 
& 0.5 & & 82.72\stdv{1.86} & 74.60\stdv{1.83} & 76.29\stdv{3.09} & 82.38\stdv{1.42} & 72.70\stdv{0.75} & \textbf{94.27}\stdv{0.71} & 93.36\stdv{0.45} & xxx\stdv{xxx} & xxx\stdv{xxx} & xxx\stdv{xxx} & xxx\stdv{xxx} 
\\
& 1.0 & & 92.42\stdv{0.20} & 86.65\stdv{1.21} & 90.88\stdv{0.82} & 91.66\stdv{0.23} & 86.81\stdv{0.72} & \textbf{96.50}\stdv{0.41} & 96.09\stdv{0.53} & xxx\stdv{xxx} & xxx\stdv{xxx} & xxx\stdv{xxx} & xxx\stdv{xxx} 
\\
& 2.0 & & 95.44\stdv{0.39} & 66.96\stdv{16.62} & 94.69\stdv{0.39} & 95.29\stdv{0.44} & 92.85\stdv{0.58} & 97.21\stdv{0.10} & \textbf{97.26}\stdv{0.19}& xxx\stdv{xxx} & xxx\stdv{xxx} & xxx\stdv{xxx} & xxx\stdv{xxx} 
\\
& 5.0 & & 97.64\stdv{0.06} & 97.08\stdv{0.30} & 97.60\stdv{0.08} & 97.61\stdv{0.10} & 96.82\stdv{0.15} & 98.12\stdv{0.27} & \textbf{98.36}\stdv{0.13} & xxx\stdv{xxx} & xxx\stdv{xxx} & xxx\stdv{xxx} & xxx\stdv{xxx} 
\\
\midrule
\multirow{4}{*}{\makecell{Corrupted CIFAR-10}} 
& 0.5 & & 22.74\stdv{0.60} & 22.22\stdv{0.87} & 22.27\stdv{0.31} & 22.94\stdv{0.41} & 21.72\stdv{0.6} & 28.14\stdv{0.61} & \textbf{30.43}\stdv{2.35}  & xxx\stdv{xxx} & xxx\stdv{xxx} & xxx\stdv{xxx} & xxx\stdv{xxx} 
\\
& 1.0 & & 25.97\stdv{0.36} & 24.83\stdv{0.44} & 26.27\stdv{0.31} & 25.86\stdv{0.37} & 25.61\stdv{0.19} & \textbf{33.07}\stdv{0.78} & 32.96\stdv{3.67} & xxx\stdv{xxx} & xxx\stdv{xxx} & xxx\stdv{xxx} & xxx\stdv{xxx} 
\\
& 2.0 & & 31.28\stdv{0.69} & 29.98\stdv{0.55} & 31.03\stdv{0.26} & 31.46\stdv{0.67} & 31.88\stdv{0.23} & 39.69\stdv{1.03} & \textbf{40.44}\stdv{1.94} & xxx\stdv{xxx} & xxx\stdv{xxx} & xxx\stdv{xxx} & xxx\stdv{xxx} 
\\
& 5.0 & & 41.58\stdv{0.33} & 40.83\stdv{0.23} & 42.35\stdv{0.45} & 41.39\stdv{0.54} & 43.07\stdv{0.41} & 48.93\stdv{0.35} & \textbf{49.34}\stdv{1.42} & xxx\stdv{xxx} & xxx\stdv{xxx} & xxx\stdv{xxx} & xxx\stdv{xxx} 
\\ 
\midrule
\multirow{4}{*}{\makecell{BFFHQ}} 
& 0.5 & & 55.64\stdv{0.44} & 56.96\stdv{0.62} & 56.88\stdv{1.13} & 55.96\stdv{0.91} & 55.76\stdv{1.5} & \textbf{65.19}\stdv{3.23} & 62.08\stdv{3.89} & xxx\stdv{xxx} & xxx\stdv{xxx} & xxx\stdv{xxx} & xxx\stdv{xxx} 
\\
& 1.0 & & 60.96\stdv{1.00} & 62.32\stdv{1.21} & 62.64\stdv{0.99} & 60.88\stdv{1.17} & 60.68\stdv{1.24} & \textbf{69.04}\stdv{2.35} & 66.00\stdv{1.33} & xxx\stdv{xxx} & xxx\stdv{xxx} & xxx\stdv{xxx} & xxx\stdv{xxx} 
\\
& 2.0 & & 69.00\stdv{0.5} & 70.72\stdv{0.89} & 69.8\stdv{1.03} & 69.72\stdv{1.14} & 69.6\stdv{1.33} & \textbf{73.08}\stdv{2.70} & 69.92\stdv{2.72} & xxx\stdv{xxx} & xxx\stdv{xxx} & xxx\stdv{xxx} & xxx\stdv{xxx} 
\\
& 5.0 & & 82.88\stdv{0.49} & \textbf{83.4}\stdv{0.34} & 83.08\stdv{0.93} & 82.88\stdv{0.74} & 82.64\stdv{0.64} & 79.8\stdv{1.09} & 80.68\stdv{0.25} & xxx\stdv{xxx} & xxx\stdv{xxx} & xxx\stdv{xxx} & xxx\stdv{xxx} 
\\
\midrule
\multirow{2}{*}{\makecell{Dogs \& Cats}} 
& 1.0 & & 48.06\stdv{7.09} & 46.76\stdv{5.3} & 50.9\stdv{4.62} & 48.56\stdv{5.69} & 48.7\stdv{6.05} & \textbf{73.1}\stdv{3.60} & 65.74\stdv{3.31} & xxx\stdv{xxx} & xxx\stdv{xxx} & xxx\stdv{xxx} & xxx\stdv{xxx} 
\\
& 5.0 & & 69.88\stdv{1.73} & 72.60\stdv{3.01} & 73.96\stdv{1.86}& 68.24\stdv{2.24}  & 65.74\stdv{0.51} & \textbf{84.32}\stdv{1.87} & 81.58\stdv{2.44} & xxx\stdv{xxx} & xxx\stdv{xxx} & xxx\stdv{xxx} & xxx\stdv{xxx} 
\\
\bottomrule
\end{tabular}}
\caption{Image classification accuracy on test sets. We added BE on LfF, DisEnt, and SoftCon which leverage a biased model for reweighting data samples. }
\label{tab:appendix_best_test}
\end{center}
\end{table}
