# Supplementary material for: Revisiting the Importance of Amplifying Bias for Debiasing
Source: arXiv:2205.14594 source file (2022-12-07)
Supplement: Supplementary file 3 [file supp_JTT.tex]

\begin{table}[t]
\centering
% \vspace{-0.1cm}
\resizebox{1.0\linewidth}{!}{
\begin{tabular}{c | c c c c}
% \hline\noalign{\smallskip}
\toprule 
Method & Colored MNIST & BFFHQ & Dogs \& Cats & BAR \\
\midrule
JTT~\cite{jtt} & 74.36\stdv{5.06} & 60.78\stdv{2.62} & 66.38\stdv{8.22} & 71.70\stdv{0.53} \\
\midrule
\multirow{2}{*}{JTT + Ours} & \textbf{78.88}\stdv{2.64} & \textbf{64.96}\stdv{1.50} & \textbf{82.91}\stdv{1.97} & \textbf{73.32}\stdv{0.53} \\ 
 & \cellcolor{Gray} (+4.52) & \cellcolor{Gray} (+4.18) & \cellcolor{Gray} (+16.53) & \cellcolor{Gray}(+1.62) \\

\bottomrule
\end{tabular}}
\vspace{-0.2cm}
\caption{ Comparisons of unbiased test set accuracies of JTT trained with and without our approach. We use 1\% ratio of bias-conflicting samples for each dataset. The performance improvements are shaded in grey.
}
\label{tab:supp_JTT}
\end{table}
